# Supplementary material for: Geometric Shaping of 2-Dimensional Constellations in the Presence of Laser Phase Noise
Source: arXiv:2007.10473 source file (2020-07-20)
Supplement: Supplementary file 1 [file Appendix.tex]

\appendix[Post-FEC Results for 32- and 64-\textit{ary} Constellations]
%\section{Appendix}
\label{sec:Appendix}
Post-FEC results for 32- and 64-\textit{ary} constellations. We observe that, as for 8- and 16-\textit{ary} constellations, the post-FEC performance is highly correlated with the GMI results.

\begin{figure}[t]
        \centering
        \begin{minipage}{0.23\textwidth}
            \centering
            \scalebox{.96}{
            \includegraphics[width=\textwidth]{32QAM/Curves/SD_Hamming_M=32_RPN=1.0e-04.tikz}} 
        \end{minipage}%
        \begin{minipage}{0.23\textwidth}
            \centering
             \scalebox{.96}{
            \includegraphics[width=\textwidth]{32QAM/Curves/SD_Hamming_M=32_RPN=2.1e-04.tikz}}\hfill
        \end{minipage}%
        \centering
        \vspace{.1cm}
        \begin{minipage}{0.23\textwidth}
            \centering
            \scalebox{.96}{
            \includegraphics[width=\textwidth]{32QAM/Curves/SD_Hamming_M=32_RPN=4.2e-04.tikz}}
        \end{minipage}%
        % \begin{minipage}{0.23\textwidth}
        %     \centering
        %     \scalebox{.93}{
        %     \includegraphics[width=\textwidth]{32QAM/Curves/dSNR_fec.tikz}}\hfill
        % \end{minipage}%
        %
        \caption{SD Hamming(128, 120) post-FEC performance for 60~Gbaud, 32-\textit{ary} constellations assuming (a) a 1~MHz, (b) a 2~MHz and (c) a 4~MHz combined laser linewidths. (d) SNR penalty vs. phase noise variance at the post-FEC threshold of $4.5\cdot 10^{-3}$.}
        \label{fig:fec_curves_32}
        % \vspace{-12pt}
\end{figure}
\begin{figure}[t]
        \centering
        \begin{minipage}{0.23\textwidth}
            \centering
            \scalebox{.96}{
            \includegraphics[width=\textwidth]{64QAM/Curves/SD_Hamming_M=64_RPN=1.0e-04.tikz}} 
        \end{minipage}%
        \begin{minipage}{0.23\textwidth}
            \centering
             \scalebox{.96}{
            \includegraphics[width=\textwidth]{64QAM/Curves/SD_Hamming_M=64_RPN=2.1e-04.tikz}}\hfill
        \end{minipage}%
        \centering
        \vspace{.1cm}
        \begin{minipage}{0.23\textwidth}
            \centering
            \scalebox{.96}{
            \includegraphics[width=\textwidth]{64QAM/Curves/SD_Hamming_M=64_RPN=4.2e-04.tikz}}
        \end{minipage}%
        % \begin{minipage}{0.23\textwidth}
        %     \centering
        %     \scalebox{.93}{
        %     \includegraphics[width=\textwidth]{64QAM/Curves/dSNR_fec.tikz}}\hfill
        % \end{minipage}%
        %
        \caption{SD Hamming(128, 120) post-FEC performance for 60~Gbaud, 64-\textit{ary} constellations assuming (a) a 1~MHz, (b) a 2~MHz and (c) a 4~MHz combined laser linewidths. (d) SNR penalty vs. phase noise variance at the post-FEC threshold of $4.5\cdot 10^{-3}$.}
        \label{fig:fec_curves_64}
        \vspace{-12pt}
\end{figure}
